# Supplementary material for: Probing breakdown of topological protection: Filling-factor-dependent evolution of robust quantum Hall incompressible phases
Source: arXiv:1812.10035 source file (2019-12-02)
Supplement: Supplementary file 1 [file Supplementary_.pdf]

# Probing breakdown of topological protection: Filling-factor-dependent evolution of robust quantum Hall incompressible phases

T. Tomimatsu,[1] K. Hashimoto,[1,2,*] S. Taninaka,[1] S. Nomura,[3] and Y. Hirayama[1,2,4]

[1]*Graduate School of Sciences, Tohoku University, Sendai 980-8578, Japan*

[2]*Centre for Spintronics Research Network, Tohoku University, Sendai 980-8578, Japan*

[3]*Division of Physics, University of Tsukuba, Tennodai, Tsukuba 305-8571, Japan*

[4]*Center for Science and Innovation in Spintronics (Core Research Cluster), Tohoku University, Sendai 980-8577, Japan*

(Dated: December 1, 2019)

## 1. Compensating for the potential mismatches between the tip and the sample

To minimize the electrostatic influence of the tip, we examined the tip-induced influence on $V_x$ modified ($\Delta V$) at different DC tip voltages ($V_{\mathrm{tip}}$) at a magnetic field of $B = 0$ T. Figure S1 shows the averaged $\Delta V$ line profiles ($\overline{\Delta V}$) taken across the Hall bar. A negative (positive) increase in $V_{\mathrm{tip}}$ decreased (increased) the electron density of the two-dimensional electron system (2DES) and therefore led $\overline{\Delta V}$ to a rise (drop) in the Hall bar (position: approximately 7–17 $\mu$m). The influence of the tip was almost completely suppressed at $V_{\mathrm{tip}} =$ 0.2 V. Compared to this compensation voltage, the imposed voltage within the measurement region was less than 0.15 mV and therefore negligibly smaller. Consequently, $V_{\mathrm{tip}} = 0.2$ V compensated for the contact potential mismatch between the tip and the 2DES. Thus, all SGM measurements were performed at $V_{\mathrm{tip}} \sim 0.2$ V.

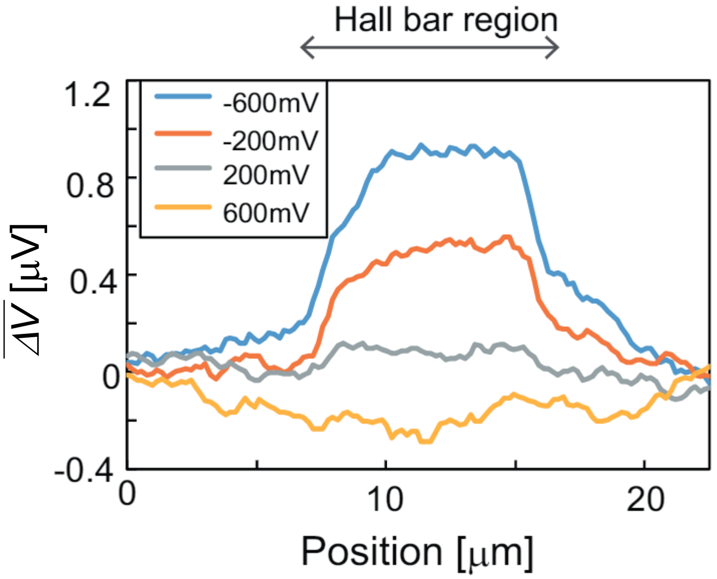


FIG. S1. **DC-tip-voltage dependence of the line profile across the Hall bar** [replotted from Ref. [1]; used in accordance with the Creative Commons Attribution (CC BY) license]. $\overline{\Delta V}$ profiles recorded at $B = 0$ T, $I_{\mathrm{sd}} = 2$ $\mu$A, and an electron density $n_{\mathrm{s}} = 1.7 \times 10^{15}$ $m^{-2}$. The value of $V_{\mathrm{tip}}$ (-600, -200, 200, and 600 mV) are indicated in the figure. The profile of each line was obtained by spatial averaging over the 9.5-$\mu m$ region in the Hall bar's longitudinal direction.

## 2. Nonequilibrium-transport-assisted scanning gate imaging

### 2.1.Nonequilibrium transport

To address the quantum Hall (QH) states near the exact integer filling factor $\nu$ ($i$) and obtain a local signal without applying a large tip voltage, we incorporated nonequilibrium transport into the SGM measurement. The application of the large $I_{\mathrm{sd}}$ leads to a nonequilibrium Hall voltage. The imposed Hall voltage predominantly enhances the potential slope [2] and drives the inter-Landau-level(inter-LL) scattering within the innermost incompressible region, which is basically insulating without the imposed $I_{\mathrm{sd}}$. The resultant non-equilibrium longitudinal voltage was used for scanning gate detection.

### 2.2. Scanning gate imaging at $\nu > i$

When the bulk filling factor $\nu$ is higher than the integer filling factor ($i$), alternating compressible and incompressible strips form along an edge of the Hall bar. This is schematically depicted in Fig. S2; the $\nu_{\mathrm{L}} = i$ incompressible region separates the $\nu_{\mathrm{L}} < i$ edge region from the $\nu > i$ bulk region. In the bulk region, electrons slightly occupy the upper LL and partially screen the disorder potential, inducing compressible areas.

The imposed nonequilibrium Hall voltage leads to an imbalance in the potential that is predominantly between neighboring compressible regions separated by the innermost incompressible edge strip [2]; the Fermi energy at the edge ($E_{\mathrm{f,edge}}$) deviates from the bulk Fermi energy ($E_{\mathrm{f}}$). This nonequilibrium potential causes inter-LL tunneling through the innermost incompressible strip into the compressible area in the interior. Then, an electron is backscattered into the opposite edge channel through compressible or directional-hopping channels along the Hall electric field. This leads to a dissipative current [2–4] and thus a nonzero longitudinal resistance. In our measurement setup (see Section 1), the average contact potential difference is canceled by applying $V_{\mathrm{tip}} = 0.2$ V. Therefore, the residual contact potential difference, namely, the effective potential mismatch, between the tip and the 2DES is solely determined by the local deviation from the average chemical potential within the

sample. In the nonequilibrium condition, the imposed excess Hall voltage deviates the local chemical potential from the ground level of the 2DES, rearranging the effective potential mismatch with the tip. The resulting nonzero potential mismatch induces a local electric field under the tip and therefore locally bends the LL, as shown in Fig. S2. The tip-induced LL bending results in a partial reduction in the neighboring LL separation ($d$) by $\delta$. The resulting tunneling current is strongly enhanced owing to its nonlinear characteristic, as expressed by $I_{\mathrm{t}} \propto e^{-(d-\delta)^2/l_B^2}$ ($l_B$: magnetic length), increasing inter-LL scattering and hence $V_{\mathrm{x}}$.

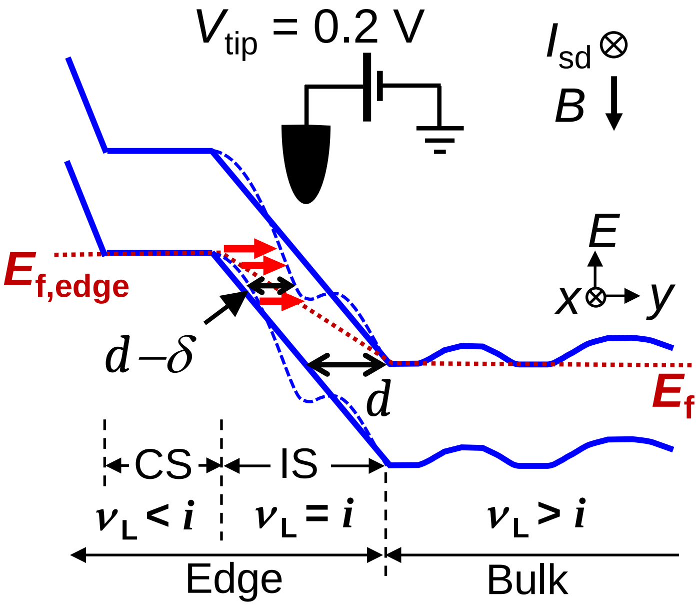


FIG. S2. **Schematic of inter-LL tunneling enhanced by the tip.** The blue dashed lines indicate the LLs that are modified from the pristine LLs (blue solid lines) by tip perturbation. The tunneling distance ($d$) locally reduces to $d - \delta$. The resultant enhancement in inter-LL tunneling at the tunneling current ($I_{\mathrm{t}}$) is indicated by the red arrows. The orange dotted line indicates the chemical potential ($E_{\mathrm{f}}$).

### 2.3. Scanning gate imaging at $\nu \simeq i$

Close to the integer filling factor $\nu = i$, the innermost incompressible strips that appear when $\nu > i$ now move and widen into the bulk region. The resultant bulk region is basically

incompressible, whereas a small deviation from $\nu = i$ at $\nu = i + \delta$ ($\nu = i - \delta$) introduces electrons (holes) into the upper empty (fully occupied) LL within a potential valley (hill), inducing compressible puddles isolated each other by the incompressible region. For the compressible puddle formed at $\nu = i + \delta$ [Fig. 4(f)], the inner compressible area with $\nu > i$ and an outer compressible area with $\nu < i$ are separated by the well-developed incompressible area where the potential has a slope. This potential slope is enhanced by the imposed nonequilibrium Hall voltage. Eventually, electron tunneling takes place from the edge compressible channel on the higher chemical potential side to the compressible puddle across the potential slope, followed by directional hoping along the Hall electric field. In the same manner as that discussed in Subsection 2.2, the tip-induced LL bending, particularly on the steepest potential slope, enhances $V_{\mathrm{x}}$, visualizing the incompressible area enclosing the compressible puddle.

### 2.4. Scanning gate imaging in the deep QH breakdown regime

An increase in the current towards the deep QH breakdown condition almost fully opens the channel across the innermost incompressible region . Moreover, the large current enhances the heating effect, which reduces the compressibility [5, 6], such that the bare disorder and confinement potentials can no longer be screened. Thus, the current is limited to hopping across the unscreened potentials. Then, the tip modifies the hopping within the interior, resulting in SGM patterns with no $\nu$ dependence that visualize the bare potential disorder, as shown in Figs. 4(d) and (e).

## 3. Dependence of the edge strip pattern on the direction of the current in the magnetic field

Figure S3 shows SGM images taken at $\nu = 1.03$ and $B = 8$ T. The edge pattern appears along the higher chemical potential $\mu_{\mathrm{high}}$ edge, which was determined to be the left (right) side of the Hall bar when $I_{\mathrm{sd}}$ is imposed in the direction indicated by the up (down) arrow.

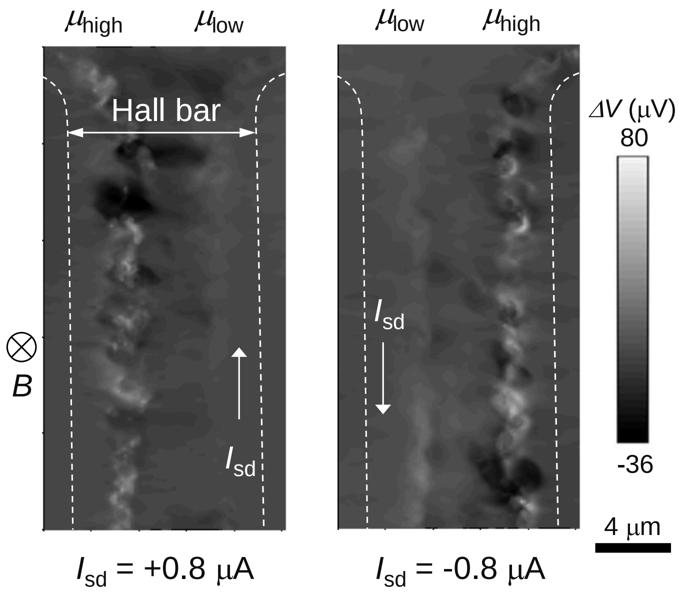


FIG. S3. **Dependence of the edge strip pattern on the direction of the current.** The edge pattern obtained at $\nu = 1.03$ and $B = 8$ T and in opposite $I_{sd}$ directions are indicated by arrows: $I_{sd} = +0.8\mu$A (left) and $-0.8\mu$A (right). $\mu_{high}$ and $\mu_{low}$ mark the higher and lower chemical potential sides, respectively.

**4.Influence of the current on the incompressible strip pattern**

We carefully selected $I_{sd}$ to minimize its influence on the incompressible strip patterns. Figures S4(a)–(b) show the current-dependent evolution of the incompressible strip at $\nu =$ 2.27 and 2.10. At $\nu = 2.27$ (Fig. S4(a)), the position of strip is rigid over the measurement range of $I_{sd}$, whereas the strip at $\nu = 2.10$ (Fig. S4(b)) shifts and widens predominantly toward the interior of the 2DES. For a quantitative comparison, we measured the position ($y_k$) of the incompressible strip, defined as a first moment in an averaged $\Delta V$ profile ($\overline{\Delta V}$), described in Section 6. The resultant $I_{sd}$ dependence of $y_k$ obtained at $\nu = 2.10$, 2.17, and 2.27 is shown in Fig. S4(c). Here, $y_k$ is almost constant over the entire range of $I_{sd}$ at $\nu = 2.17$ and 2.27. At $\nu = 2.10$, however, it increases for a current above $I_{sd}$= 4 $\mu$A. Thus, we limited $I_{sd}$ below 4 $\mu$A to obtain unperturbed incompressible strips.

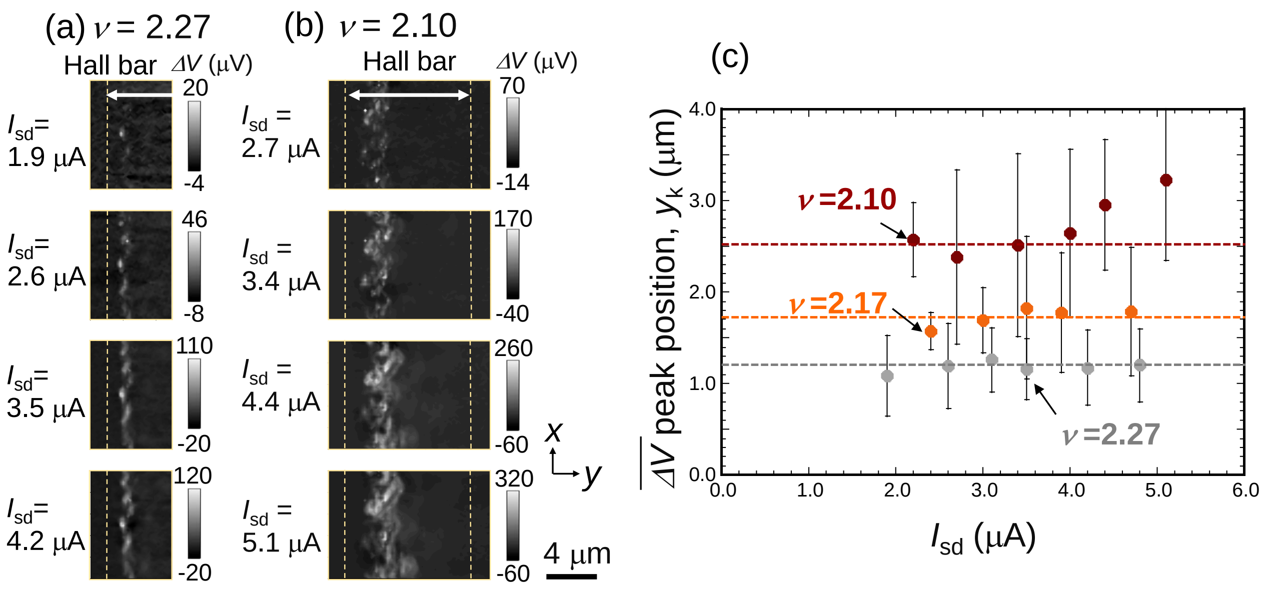


FIG. S4. **Influence of the current on the incompressible patterns.** (a), (b) Comparison of SGM images for different $I_{\rm sd}$ at $B = 4$ T and (a) $\nu = 2.27$ and (b) $\nu = 2.10$ . (c) Influence of the current on the $\overline{\Delta V}$ peak positions measured from the Hall bar edge ($y_{\rm k}$) for $\nu$ =2.10, 2.17, and 2.27.

## 5. Nonequilibrium condition for SGM measurement

Figure S5(a) displays the color-scale $I_{\rm sd}$–$\nu$ plots of the longitudinal voltage ($V_{\rm x}$) measured at $B = 4$ T near $\nu = 2$. The dissipation-less integer QH state represented by $V_{\rm x} \simeq 0$ (dark blue area) breaks down with an abrupt increase in $V_{\rm x}$ with $I_{\rm sd}$. The points marked by red dots indicate the measurement conditions for Fig. 2(c), including Fig. 2(a). Here, we tuned $I_{\rm sd}$ at different $\nu$ to maintain $V_{\rm x}$ unperturbed by the tip, i.e., $V_{\rm x}$ obtained as the tip was positioned outside the Hall bar. This offset voltage was optimized to be $V_{\rm x} = 1.2$ mV in order to obtain a sufficient tip-induced $V_{\rm x}$ change with minimal $I_{\rm sd}$ to avoid the current-induced deformation of the incompressible strip, as described in Section 4. For $\nu_{\rm local} = 4$ ($B = 2$ T) and $\nu_{\rm local} = 1$ ($B = 8$ T), the color-scale $I_{\rm sd} - \nu$ plots of $V_{\rm x}$ as well as the measurement points chosen at the offset voltage $V_{\rm x} = 0.8$ mV are shown in Figs. S5(b) and (c).

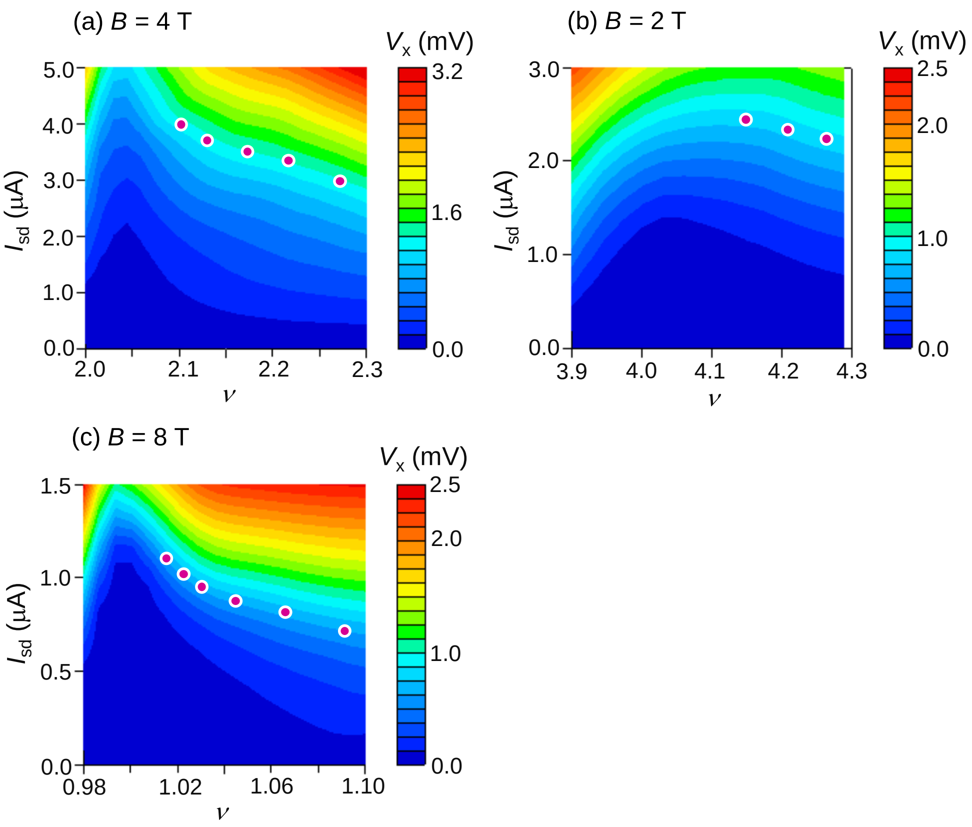


FIG. S5. **SGM condition for imaging the incompressible region for (a) $\nu_{\rm local} = 2$, (b) $\nu_{\rm local} = 4$, and (c) $\nu_{\rm local} = 1$.** The red solid circles indicate $I_{\rm sd}$ used for the corresponding measurements [Figs. 2 and 3]. Here, $I_{\rm sd}$ was selected such that the corresponding $V_{\rm x}$ without tip perturbation is approximately constant, as indicated by the superposed color-scale plots of the unperturbed $V_{\rm x}$.

## 6. Determining the positions and widths of the SGM line patterns

To determine the positions and widths of the line patterns, we first averaged the $\Delta V$ profile over the 8.5-$\mu m$ range in the Hall bar's longitudinal ($x$) direction and then plotted the resulting $\overline{\Delta V}$ profile as shown in Fig. S6. Then, we measured the full width at half maximum, $W_{\rm FWHM} = y_2 - y_1$, of the peak in the $\overline{\Delta V}$ profile and finally the first moment ($y_{\rm k}$) in the $\overline{\Delta V}$ profile. Here, $y_{\rm k}$ is

$$y_{\rm k} = \frac{\int_{y_1}^{y_2} y \cdot \overline{\Delta V(y)} dy}{\int_{y_1}^{y_2} \overline{\Delta V(y)} dy} \tag{1}$$

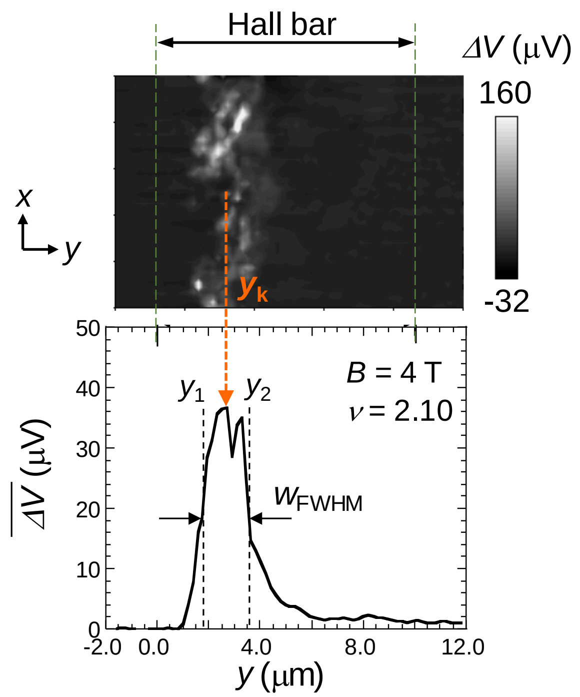


FIG. S6. **Position and width of the $\Delta V$ peak.** The upper panel shows the SGM image taken at $\nu = 2.10$, $I_{\mathrm{sd}} = 4$ $\mu$A, and $B = 4$ T. The lower panel shows the $\overline{\Delta V}$ profile obtained by averaging $\Delta V$ over the 8.5-$\mu$m range in the $x$ direction extracted from the SGM image (upper panel).

### 7. Local spin-density approximation

To calculate the position and width of the spin-resolved incompressible strips in the QH regime ($I_{\mathrm{sd}} = 0$ A), we used the local spin-density approximation (LSDA) [7, 8]. The Hamiltonian comprised the kinetic energy in the Landau gauge, the confinement potential, the Hartree term, the exchange energy term, and the Zeeman term. The wave functions were calculated on three-dimensional (3D) grids $x \times z \times k_{\mathrm{y}}$ of $1158 \times 6 \times 387$, $1521 \times 6 \times 507$, and $2151 \times 6 \times 717$, at 2, 4, and 8 T, respectively, where $k_{\mathrm{y}}$ is the wave vector in the $y$ direction, with the size of the unit cell of the real-space grid, $(l_{\mathrm{B}}/3)^2$, where $l_{\mathrm{B}}$ is the magnetic length. The potentials were calculated on 2D grids of $1158 \times 47$, $1521 \times 47$, and $2151 \times 47$, at 2, 4, and 8 T, respectively, per unit cell. We considered a 6-$\mu$m-wide quantum wire to calculate the electronic structure on the half side of the 10-$\mu$m-wide Hall bar used for the measurements. As the lateral confinement potential, we incorporate the edge potential of an ellipsoid, which has been widely used to analyze the edge's electronic structure [9, 10]:

$V_c = V_0(y) + V_{c0}(1 - \sqrt{1 - [(y - y_0)/y_1]^2})$, where both the center $y_0$ and the half-width $y_1$ of the Hall bar are $y_0 = y_1 = 5$ $\mu$m. Here, $V_0$ (the potential barrier outside the Hall bar) and $V_{c0}$ were assumed to be $V_0 = 1000$ eV ($y < 0$ $\mu$m and $y > 6$ $\mu$m; otherwise, $V_0 = 0$ eV) and $V_{c0} = 0.17$ eV, respectively. The temperature was $T = 0.5$ K. Details regarding this calculation, including the material parameters for GaAs and GaAlAs, can be found elsewhere [8].

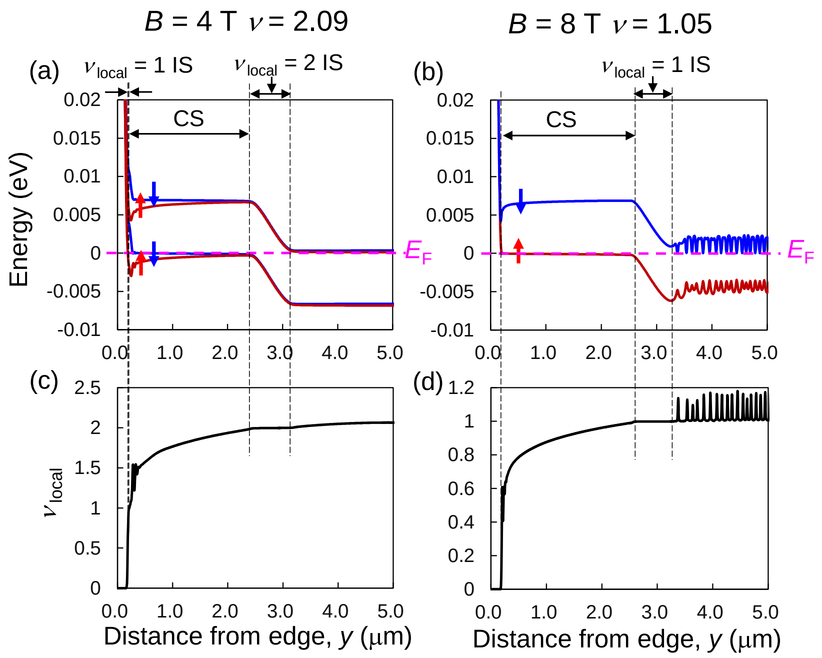


FIG. S7. **Subband structures and electron density profiles obtained with the LSDA.** Calculated subband structures at (a) $\nu = 2.09$ and $B = 4$ T and (b) $\nu = 1.05$ and $B = 8$ T. Calculated lateral electron density profiles for (c) $\nu = 2.09$ and $B = 4$ T and (d) $\nu = 1.05$ and $B = 8$ T. Incompressible and compressible strips are denoted "IS" and "CS," respectively. An oscillatory structure in the compressible region ($y > 3.3\mu m$) is caused by oscillating populations for spin-up and spin-down electrons owing to the exchange interaction[11].

The calculated subband structures for $\nu = 2.09$ and $B = 4$ T and for $\nu = 1.05$ and $B = 8$ T are depicted in Figs. S7(a) and (b), respectively. At $\nu = 2.09$ (Fig. S7(a)), the spin-up and spin-down levels degenerate in the region away from the $\nu_{\text{local}} = 1$ incompressible strip. By contrast, at $\nu = 1.05$ (Fig. S7(b)), the degeneracy of the spin subbands is lifted over the entire region of the 2DES by the exchange enhancement. The LL in the incompressible region slopes owing to poor screening, whereas the LL in the compressible region becomes

nearly flat. The corresponding electron density profiles show a constant density in the incompressible strips when $\nu_{\rm local} = 1$ and 2 (Fig. S7(c)) and $\nu_{\rm local} = 1$ (Fig. S7(d)). We defined the $\nu_{\rm local}$ incompressible strip as the area where $\nu_{\rm local} = {\rm int}(\nu) \pm \delta\nu$. Here, ${\rm int}(\nu)$ indicates an integer of the LL filling factor, and $\delta\nu = \delta n_{\rm s} e/Bh$ is determined by a constant $\delta n_{\rm s} = 1.93 \times 10^{13}$ m$^{-2}$. Thus, the incompressible strips are determined as the area where $\nu_{\rm local} = 1 \pm 0.01$ at $B = 8$ T, $2 \pm 0.02$ at $B = 4$ T, and $4 \pm 0.04$ at $B = 2$ T. Note that the well-developed $\nu_{\rm local} = 1$ incompressible region is caused by the exchange enhancement of the spin-split gap, which is considered in the LSDA calculation; otherwise, the incompressible strip shrinks with a bare spin-split gap at the bare $g$-factor of 0.44.

**8. Global longitudinal and Hall resistances**

To obtain the global transport characteristics at equilibrium in the QH regime, we measured the longitudinal ($R_{\rm xx}$) and Hall ($R_{\rm xy}$) resistances using Hall-bar voltage probes at a low current $I_{\rm sd} = 10$ nA. The resulting $R_{\rm xx}$ and $R_{\rm xy}$ measured at $B = 8$ T [Fig. S8(a)], $B = 6$ T [Fig. S8(b)], $B = 4$ T [Fig. S8(c)], and $B = 2$ T [Fig. S8(d)] were plotted as a function of $\nu$. Dotted lines mark the $\nu$ positions at which the SGM images in Fig. 3(a) [Fig. S8(a)], Figs. 4(a)–(c) [Fig. S8(b)], Fig. 2(a) [Fig. S8(c)], and Fig. 2(b) [Fig. S8(d)] were captured.

**9. Supplementary Movies**

The supplementary movies show the incompressible patterns from a low current ($I_{\rm sd} =$ 0.1–0.7 $\mu$A) to a high current ($I_{\rm sd} =$ 1.7–2.5 $\mu$A) for $\nu = 1.05$, 1.01, and 0.97 at $B = 8$ T. The movie in the left (middle) panel taken at $\nu = 1.05$ ($\nu = 1.01$) displays the evolution of the incompressible pattern from the low-current image shown in Fig. 4(a) (Fig. 4(b)) to the high-current image shown in Fig. 4(d) (Fig. 4(e)). An additional movie taken at $\nu = 0.97$ is also shown in the right panel. All movies clearly demonstrate that the $\nu$ dependence of the pattern among the three filling factors completely vanishes with large $I_{\rm sd}$, implying the breakdown of the QH effect.

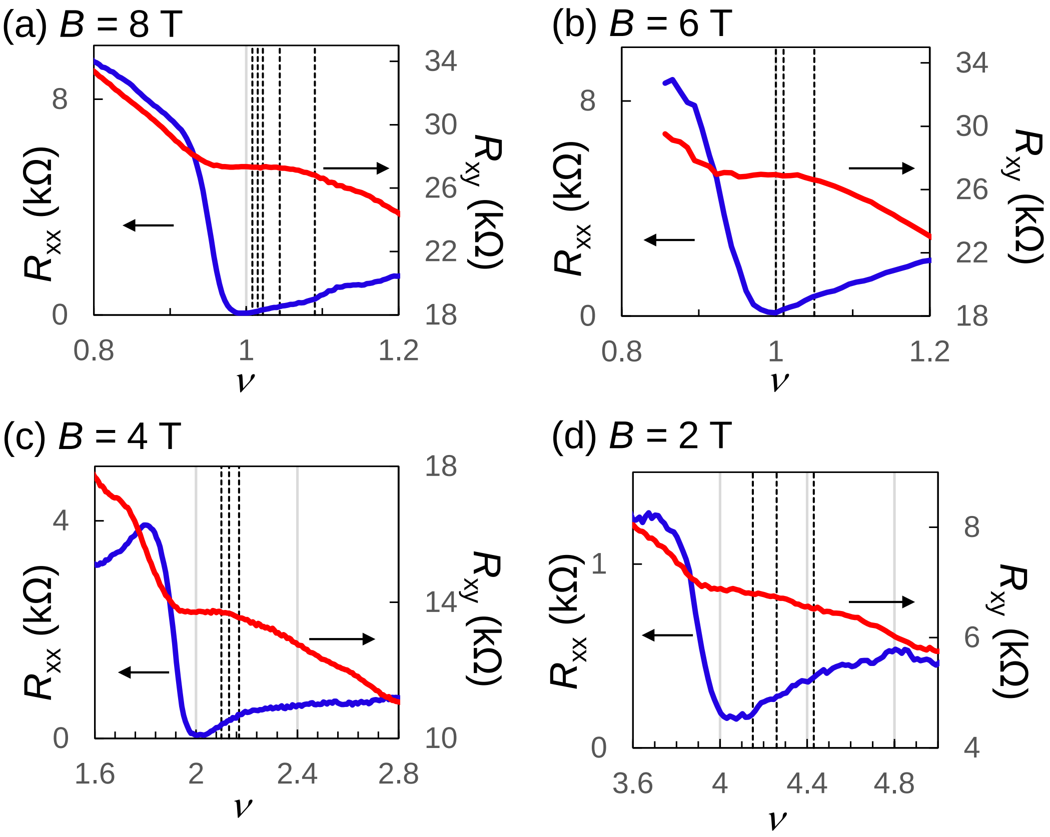


FIG. S8. **Comparison of global transport measurements and scanning gate imaging.** (a)–(d) Longitudinal ($R_{\rm xx}$) and Hall($R_{\rm xy}$) resistance curves measured at (a) $B = 8$ T, (b) $B = 6$ T, (c) $B = 4$ T, and (d) $B = 2$ T. Dotted lines mark the $\nu$ positions at which the SGM images in Fig. 3(a) [Fig. S8(a)], Figs. 4(a)–(c) [Fig. S8(b)], Fig. 2(a) [Fig. S8(c)], and Fig. 2(b) [Fig. S8(d)] were captured.

* hashi@tohoku.ac.jp

[1] K. Hashimoto, T. Tomimatsu, K. Sato, and Y. Hirayama, Nature Communications **9**, 2215 (2018).

[2] J. Weis and K. V. Klitzing, Philosophical Transactions of the Royal Society A: Mathematical, Physical and Engineering Sciences **369**, 3954 (2011).

[3] L. Eaves and F. W. Sheard, Semiconductor Science and Technology **1**, 346 (1986).

[4] K. Panos, R. Gerhardts, J. Weis, and K. von Klitzing, New Journal of Physics **16**, 113071 (2014).

[5] T. Machida, H. Hirai, S. Komiyama, T. Osada, and Y. Shiraki, Phys. Rev. B **54**, 14261 (1996).

[6] M. Kato, A. Endo, S. Katsumoto, and Y. Iye, Physical Review Letters **102**, 086802 (2009).

[7] S. Nomura and Y. Aoyagi, Physical Review Letters **93**, 096803 (2004).

[8] S. Mamyouda, H. Ito, Y. Shibata, S. Kashiwaya, M. Yamaguchi, T. Akazaki, H. Tamura, Y. Ootuka, and S. Nomura, Nano Letters **15**, 2417 (2015).

[9] D. B. Chklovskii, B. I. Shklovskii, and L. I. Glazman, Physical Review B **46**, 4026 (1992).

[10] K. Güven and R. R. Gerhardts, Physical Review B **67**, 115327 (2003).

[11] S. Ihnatsenka and I. V. Zozoulenko, Physical Review B **73**, 155314 (2006).
